# Supplementary material for: Probing the interiors of the ice giants: Shock compression of water to 700 GPa and 3.8 g/ccm
Source: arXiv:1201.2622 ancillary file (2012-01-12)
Supplement: Supplementary file 1 [file supplement.pdf]

# Probing the interiors of the ice giants:

# Shock compression of water to 700 GPa and 3.8 g/cc

M.D. Knudson, M.P. Desjarlais, R.W. Lemke, and T.R. Mattsson

*Sandia National Laboratories, Albuquerque, NM, USA*

M. French, N. Nettelmann, and R. Redmer

*Institut für Physik, Universität Rostock, D-18051 Rostock, Germany*

## Supplemental Material

The 6061-T6 aluminum flyer-plates were 17-by-44 mm in lateral dimension and initially 1 mm in thickness. However, due to magnetic field diffusion associated with the magnetic acceleration of the plate, at the time of impact a significant portion of the original flyer-plate thickness was at densities below ambient. This effect has been extensively studied, both through experiment and magneto-hydrodynamic simulation, and is well understood [1]. In particular, for the flyer-plate configurations used in this work, a few to several hundred microns of the impact side of the aluminum flyer-plate were at ambient density, evidenced by the initially very steady shock velocities recorded in the quartz drive plate and water samples, as shown in Supplemental Fig. 1. The subsequent decrease in observed shock velocity is due to a corresponding decrease in flyer-plate density, indicating the extent to which magnetic diffusion had penetrated into the flyer plate.

A water sample was contained within an aluminum water cell machined from 6061-T6 aluminum. A quartz window with a Viton o-ring was clamped to the rear of the aluminum cell to provide optical access to the water sample. In some cases (3 of the 8 measurements) an additional quartz plate (250 micron thickness) was placed between the aluminum drive plate (300 micron thickness) and the water sample (500 micron thickness). Prior to filling the cell, the sample thickness (determined by the cell gap) was measured to within ~1 to 2 microns using a through-the-lens auto focusing instrument. Environmental grade water (Fisher Scientific) was allowed to flow through the cell, flushing any contaminants, and ultimately filled the cell, thereby creating the water sample.

Typically nine independent VISAR measurements, using four different sensitivities, commonly referred to as the velocity per fringe (VPF), to resolve any $2\pi$ fringe shift ambiguities, were made for both the flyer-plate and water cell. Measurements were made with a VPF as low as ~250 m/s/fringe. We conservatively estimate that the fringe count can be resolved to 1/10 of a fringe. This results in an absolute uncertainty in the inferred velocity of ~ 0.025 km/s, which corresponds to percentage uncertainties of approximately 0.1 to 0.2% over both the impact velocity range of 12 to 27 km/s, and the quartz and water shock velocity range of 12 to 25 km/s. Weighted averaging could then be used to reduce the overall uncertainty in the measured flyer-plate and shock velocities even further. However, to be conservative we took the uncertainties to be 0.2 to 0.5%.

Impedance matching was performed using the Rankine-Hugoniot (RH) jump relations [2], a set of conditions derived by considering conservation of mass, momentum, and energy across a steady propagating shock wave, relating the initial energy $E$, volume $V$, and pressure $P$, with steady-state, post-shock values

$$(E_1 - E_0) = (P_1 + P_0)(V_0 - V_1)/2 \qquad (1)$$

$$(P_1 - P_0) = \rho_0 U_s(u_{p1} - u_{p0}) \qquad (2)$$

$$\rho_1 = \rho_0[U_s/(U_s - (u_{p1} - u_{p0}))] \qquad (3).$$

Here $\rho$, $U_s$, and $u_p$ denote the density, shock velocity, and particle velocity, respectively, and the subscripts 0 and 1 denote the initial and final values. These relations conveniently allow graphical analysis in the $P - u_p$ plane to determine kinematic values upon transmission or reflection of shock waves. Both $P$ and $u_p$ must be equal across an interface for it to remain in contact; a difference in $P$ would result in a non-zero force that would drive the interface apart, and a difference in $u_p$ would result in separation of the interfaces.

Propagation of uncertainties utilized a Monte Carlo technique to account for both random measurement errors and systematic errors in the aluminum and quartz standards [3-4]. A linear $U_s - u_p$ response was used to represent the shock response of the aluminum standard ($U_s = (6.341 \pm 0.003) + (1.185 \pm 0.002)u_p$), while a quadratic response was used for the quartz standard ($U_s = (1.56 \pm 0.30) + (1.91 \pm 0.10)u_p - (0.038 \pm 0.010)u_p^2 + (0.00070 \pm 0.00032)u_p^3$). The constants $C_0$ and $S$ ($C_0$, $S_1$, $S_2$, and $S_3$ for quartz) were represented by statistical variation about

their most probably values within the one-sigma uncertainty, taking into account correlations. Similarly, each shock velocity and flyer-plate velocity were randomly sampled within a population generated by the experimental values and one-sigma uncertainties. The complete data set was then analyzed via impedance matching to determine the shock and re-shock states of the water. This process was repeated for one million runs, and the kinematic values and uncertainties were taken to be the most probable values and the standard deviations, respectively. We note that the inferred Hugoniot state for water depends upon the release response of aluminum and quartz; the impedance of water is significantly less than the impedance of either aluminum or quartz, and thus the drive plate (either aluminum or quartz) undergoes a substantial release. The release response was determined from quantum molecular dynamics (QMD) calculations of both aluminum and quartz [3,5] to determine the correction from the simplified reflected Hugoniot approximation. The uncertainty in the correction was very conservatively taken to be half of the correction to the reflected Hugoniot. These Hugoniot data are listed in Supplemental Table I.

The reanalysis of the Podurets *et al.* datum [6], which utilized aluminum as the shock standard, followed the same procedures as that outlined above.

We used the measured shock velocity in the water immediately prior to shock break-out from the water to the rear quartz window, along with a weighted fit to the Hugoniot data using the Z data, the datum of Volkov *et al.* [7] and the two highest pressure data points of Mitchell and Nellis [8] (fit parameters of $C_0 = 2.19 \pm 0.13$

and $S = 1.35 \pm 0.01$) to determine the initial state of the water for the re-shock measurements. These values are listed in Supplemental Table II.

Another way of representing the re-shock data is to plot only the observables in the experiment, namely the shock velocity in the quartz anvil as a function of the shock velocity in water, as shown in Supplemental Fig. 2. The various EOS models can then be projected onto this plane. This method provides a more direct way to evaluate the various EOS models; comparison in the $P$ - $\rho$ plane can be problematic in that for a given shock speed in water the various EOS models would predict vastly different first shock $P$ and $\rho$ states. Furthermore, the uncertainties in the measured observables are of order a few tenths of a percent. Thus, compared in this way, these data provide a very stringent test of EOS models for water in this $P$ and $\rho$ region that is directly relevant to planetary modeling. Impedance matching was used to project the various water EOS models [9-11] onto the shock velocity in quartz versus shock velocity in water plane. Possible systematic uncertainties in the quartz Hugoniot [3] were taken into account using a Monte Carlo method similar to that described above. The result was an uncertainty in the mapping that is less than the width of the lines shown in the figure.

The adiabat for GJ436b was obtained from an interior model calculation [12] that reproduces the observational constraints for mass (23.2 ME) and radius (4.2 RE), assumes an irradiated isothermal atmosphere at 1300K, and is consistent with the predicted H/He:ice:rock ratio from formation models for this planet. Because water, if present, would be in a fluid phase in this hot Neptune, we assumed a

homogeneous mixture of water and H/He in the envelope. This model has a water mass fraction of 70% in the envelope and a rock core mass of 12 ME. As for Neptune, the $P$ - $\rho$ relation along the planetary adiabat in Figs. 2(a) and 2(b) of the main text is the partial mass density of water at given internal pressure in the envelope.

## References


1. R. W. Lemke *et al.* J. Appl. Phys. **98**, 073530 (2005).
2. G. E. Duvall and R. A. Graham, Rev. Mod. Phys. **49**, 523 (1977).
3. M. D. Knudson and M. P. Desjarlais, Phys. Rev. Lett. **103**, 225501 (2009).
4. M. D. Knudson *et al.* J. Appl. Phys. **94**, 4420 (2003).
5. M. P. Desjarlais, AiP Conf. Proc. **1161**, 32 (2009).
6. M. A. Podurets *et al.* Sov. Phys. JETP **35**, 375 (1972).
7. L. P. Volkov *et al.* JETP Lett. **31**, 513 (1980).
8. A. C. Mitchell and W. J. Nellis, J. Chem. Phys. **76**, 6273 (1982).
9. S. P. Lyon and J. D. Johnson, Technical Report No. LA-UR-92-3407, Los Alamos, 1992 (unpublished).
10. F. H. Ree, Technical Report No. UCRL-52190, Lawrence Livermore Laboratory, 1976 (unpublished).
11. M. French *et al.* Phys. Rev. B **79**, 054107 (2009).
12. N. Nettelmann et al. A & A **523**, A26 (2010).

**Supplemental Figure Captions**

Supplemental Fig. 1. Typical VISAR data. Black line, aluminum flyer-plate velocity; cyan (blue) line, quartz (water) shock velocity. Inset shows a schematic of the water cel with the additional quartz drive plate (not to scale). The VISAR data clearly show (1) flyer-plate impact with the water cell, (2) shock break-out from the aluminum drive plate to the water sample, (3) shock break-out from the aluminum to the quartz drive plate, (4) shock break-out from the quartz drive plate to the water sample, and (5) shock break-out from the water sample to the rear quartz window. Upper (lower) curves correspond to aluminum/water/quartz (aluminum/quartz/water/quartz) cell.

Supplemental Fig. 2. Quartz shock velocity as a function of water shock velocity. *Models*: (pink, gray, orange) lines, (ANEOS [9], Sesame [10 ], first-principles [11]) projections. *Data*: orange diamonds, this work.

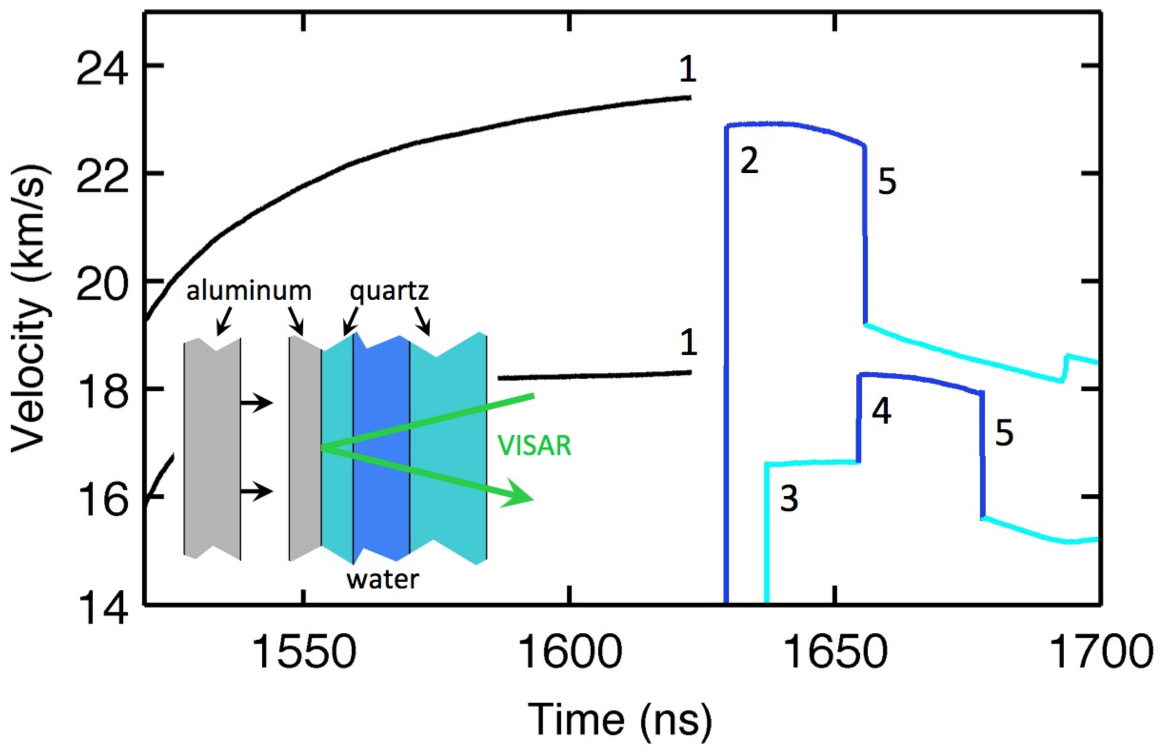


Knudson, et al., Supplemental Fig.1

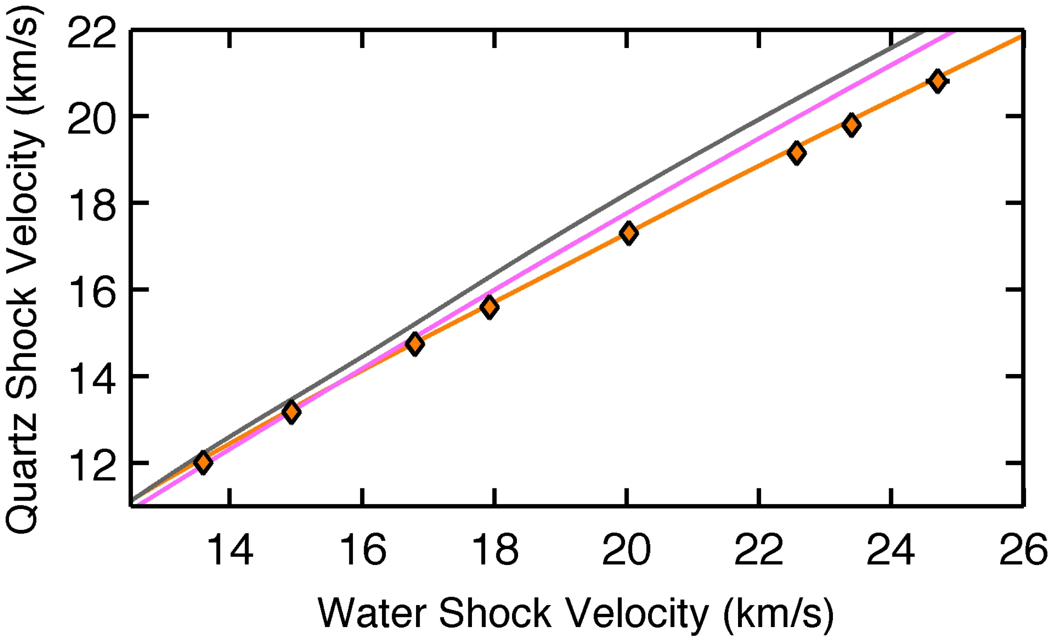


Knudson, et al., Supplemental Fig.2

## Supplemental Tables

Table I. Principal Hugoniot data for water. $v_f$ is the measured aluminum flyer-plate velocity. Values in parentheses are the one-sigma uncertainties.

| Standard | Aluminum $\boldsymbol{v_f}$ (km/s) | Quartz $\boldsymbol{U_s}$ (km/s) | Water $\boldsymbol{U_s}$ (km/s) | Water $\boldsymbol{u_p}$ (km/s) | Water $\boldsymbol{\rho_1}$ (g/cc) | Water $\boldsymbol{P_1}$ (GPa) |
|---|---|---|---|---|---|---|
| aluminum | 12.14 (0.03) | --- | 13.52 (0.03) | 8.35 (0.04) | 2.609 (0.023) | 112.6 (0.6) |
| aluminum | 14.06 (0.03) | --- | 15.02 (0.03) | 9.56 (0.04) | 2.746 (0.023) | 143.3 (0.7) |
| aluminum | 16.24 (0.03) | --- | 16.83 (0.03) | 10.91 (0.04) | 2.839 (0.023) | 183.3 (0.7) |
| quartz | --- | 16.65 (0.03) | 18.27 (0.04) | 12.01 (0.07) | 2.915 (0.030) | 219.1 (1.5) |
| quartz | --- | 18.54 (0.04) | 20.74 (0.06) | 13.74 (0.07) | 2.956 (0.038) | 284.3 (1.7) |
| aluminum | 23.40 (0.07) | --- | 22.89 (0.07) | 15.25 (0.06) | 2.991 (0.033) | 348.4 (1.6) |
| aluminum | 24.55 (0.07) | --- | 23.76 (0.07) | 15.96 (0.07) | 3.040 (0.034) | 378.4 (1.8) |
| quartz | --- | 22.20 (0.06) | 25.56 (0.15) | 17.22 (0.11) | 3.061 (0.061) | 439.3 (3.4) |
| aluminum[a] | 36.4 (0.24) | --- | 43.95 (0.30) | 31.74 (0.50) | 3.592 (0.18) | 1392 (23) |

[a] Reanalysis of the Podurets *et al.* [6] datum.

Table II. Re-shock data for water. Values in parentheses are the one-sigma uncertainties.

| Water $U_s$ (km/s) | Quartz $U_s$ (km/s) | Water $\rho_2$ (g/cc) | Water $P_2$ (GPa) |
|---|---|---|---|
| 13.60 (0.03) | 12.01 (0.03) | 3.215 (0.060) | 195.0 (1.1) |
| 14.93 (0.03) | 13.17 (0.03) | 3.296 (0.051) | 240.8 (1.2) |
| 16.80 (0.03) | 14.75 (0.03) | 3.404 (0.046) | 312.0 (1.6) |
| 17.93 (0.04) | 15.59 (0.03) | 3.522 (0.049) | 354.2 (1.7) |
| 20.03 (0.06) | 17.30 (0.05) | 3.607 (0.053) | 449.7 (3.1) |
| 22.57 (0.07) | 19.15 (0.06) | 3.794 (0.067) | 567.9 (3.9) |
| 23.40 (0.07) | 19.80 (0.06) | 3.814 (0.070) | 613.2 (4.3) |
| 24.70 (0.15) | 20.81 (0.13) | 3.843 (0.085) | 687.6 (9.5) |

Table III. Reflectivity data for water. The reflectivity values represent an average measurement encompassing the entire traversal of the shock through the water cell, therefore the reported $P$ was obtained from the average of $U_{SW}$ over the traversal of the cell. Values in parentheses are the one-sigma uncertainties.

| Water ***P*** (GPa) | Water Reflectivity |
|---|---|
| 113.7 (0.7) | 0.036 (0.027) |
| 142.0 (0.8) | 0.091 (0.030) |
| 182.4 (1.0) | 0.158 (0.041) |
| 213.9 (1.1) | 0.217 (0.043) |
| 274.2 (1.9) | 0.224 (0.044) |
| 344.2 (2.4) | 0.243 (0.055) |
| 372.7 (2.7) | 0.221 (0.060) |
| 425.5 (5.4) | 0.224 (0.075) |
